# Supplementary material for: EchoEA: Echo Information between Entities and Relations for Entity Alignment
Source: arXiv:2107.03054 source file (2021-10-25)
Supplement: Supplementary file 1 [file 070_appendix.tex]

\subsection{Open Source}
\label{sec:appendix:framework}

The source code is available at \url{https://github.com/LinXueyuanStdio/EchoEA}. We cite these projects and thank them for their great contributions!

\begin{enumerate}
  \item JAPE (MIT License):\url{https://github.com/BrianTin/JAPE}
  \item GCN-Align:\url{https://github.com/1049451037/GCN-Align}
  \item RREA:\url{https://github.com/MaoXinn/RREA}
  \item EMGCN:\url{https://github.com/thanhtrunghuynh93/EMGCN}
  \item RAGA:\url{https://github.com/zhurboo/RAGA}
\end{enumerate}
